# Supplementary material for: Negative Sampling with Adaptive Denoising Mixup for Knowledge Graph Embedding
Source: arXiv:2310.09781 source file (2023-10-15)
Supplement: Supplementary file 1 [file 7_Appendix.tex]

\appendix
\section{Toy Experiments}
We perform more toy experiments as described in Figure \ref{fig:example}(b) on multiple KGEs, such as RotatE\cite{RotatE} and TransE\cite{TransE}. As shown in Figure \ref{more-toy}, normal means normal negative sampling, and leakage means ensuring sampled negative triples are not contained in the validation or test set. In other words, we regard triples in the validation and test sets as false-negative triples during training. Compared with normal negative sampling, negative sampling with data leakage can improve the performance of KGEs. This phenomenon indicates that the bad effect of sampled noisy triples on KGEs is general. So it is important to consider the denoising issue in negative sampling for KGEs as mentioned in our paper.
\begin{figure*}[h]
    \begin{minipage}{\linewidth}
        \centering
        \centerline{\includegraphics[height=3.5cm]{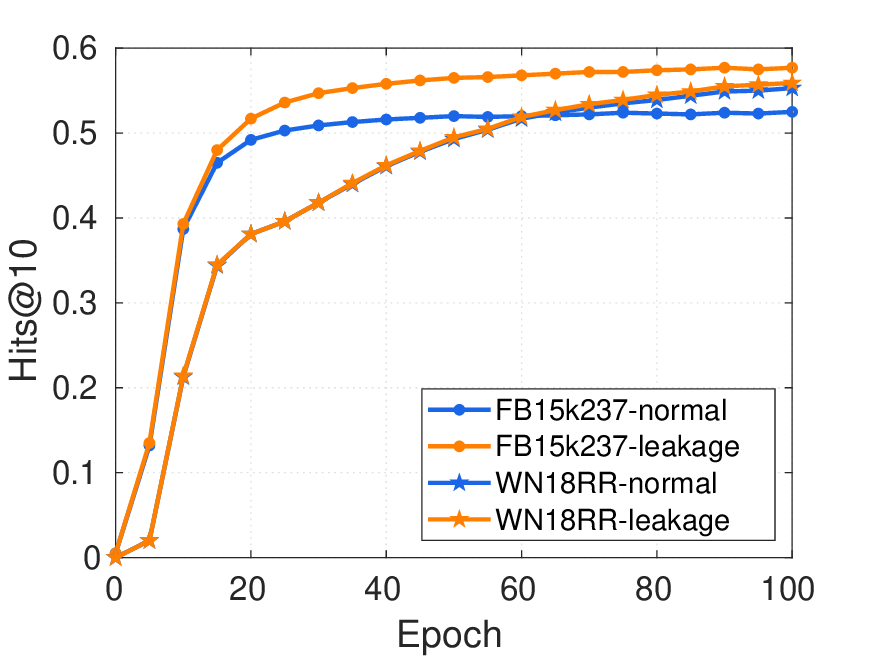}}\centerline{(a) Testing Hits@10 performance v.s. Epoch based on RotatE.}
    \end{minipage}\\
    \begin{minipage}{\linewidth}
        \centering
        \centerline{\includegraphics[height=3.5cm]{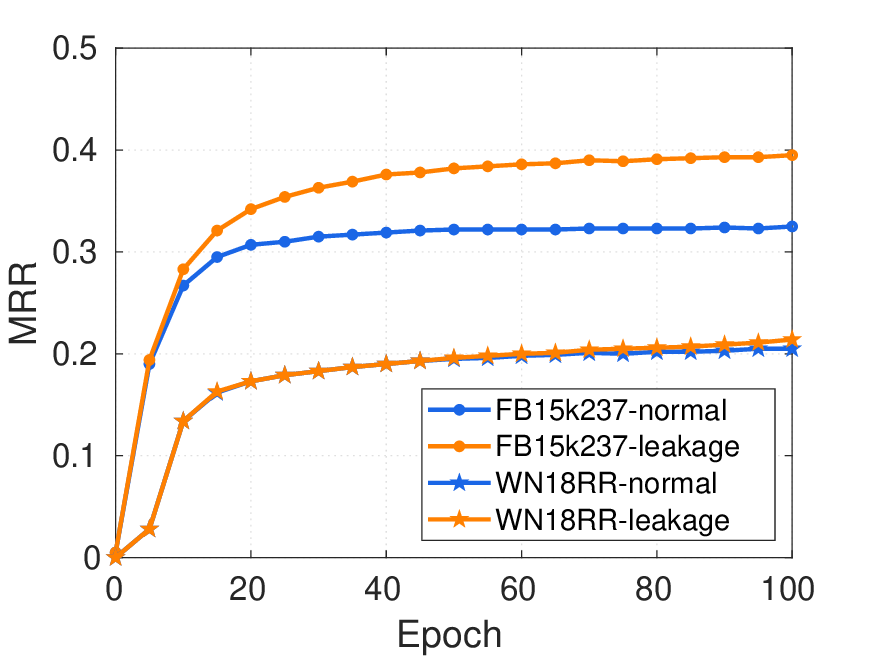}}\centerline{(b) Testing MRR performance v.s. Epoch based on TransE.}
    \end{minipage}
    \begin{minipage}{\linewidth}
        \centering
        \centerline{\includegraphics[height=3.5cm]{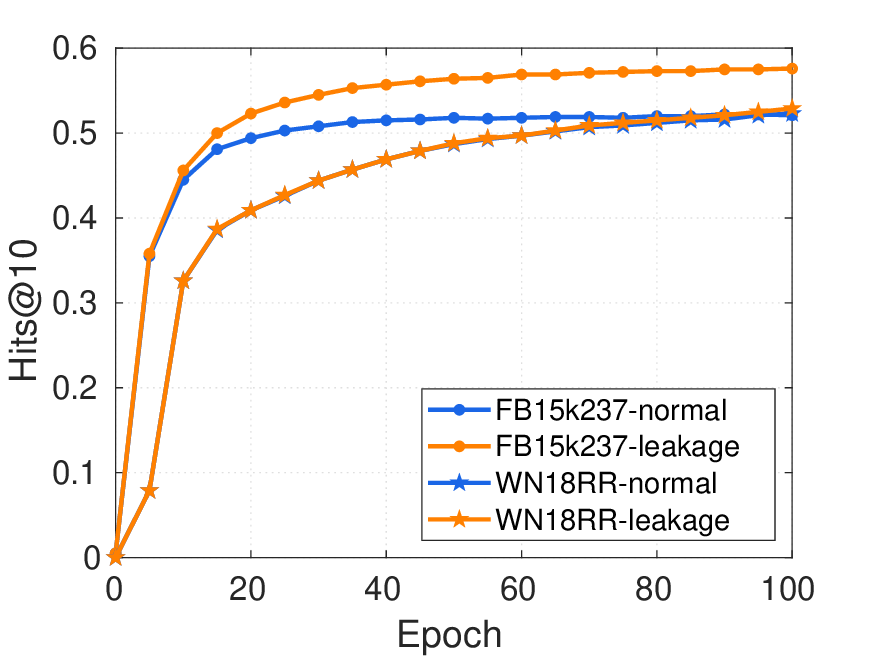}}\centerline{(c) Testing Hits@10 performance v.s. Epoch based on TransE.}
    \end{minipage}
	\caption{Toy experiments on RotatE and TransE.} 
	\label{more-toy} 
\end{figure*}
